# Supplementary material for: DLAFormer: An End-to-End Transformer For Document Layout Analysis
Source: arXiv:2405.11757 source file (2024-05-20)
Supplement: Supplementary file 1 [file appendix.tex]

\appendix
\appendixname
